# Supplementary material for: An efficient distributed learning algorithm based on effective local functional approximations
Source: arXiv:1310.8418 source file (2015-03-16)
Supplement: Supplementary file 1 [file appendix_C.tex]

\section{Appendix C: Discussion of convergence rate}
\label{appc}

\paragraph{Convergence theory}

Let us discuss further, the convergence rate assoctaed with the distributed method described in section~\ref{distr}.

We first consider the ideal case where $d_r$ is computed as a convex combination of the $\what^*_p-w^r$ where
$\what^*_p$ is the true optimum of $\fhat_p$.   It can be shown (see Appendix A, Lemma 5) that the directions $\what^*_p-w^r$ satisfy condition (1) for $\theta=\cos^{-1}\frac{\sigma}{L}$ and therefore that their convex combination $d^r$ also satisfies condition (\ref{angle}) for the same $\theta$.

Combining this with Theorem 2 implies that each round of this algorithm contracts the residual error by a factor whose absolute value is smaller than  $  (1 -  \TWO alpha(1-beta) \frac{\sigma^4}{L^4} ) < 1$ .   Note that the actual value
of the ratio $\sigma/L$ can be vastly improved by a well-chosen coordinate change on the weights $w$.  The ratio approaches $1$ when the function f is twice differentiable and the coordinate change is $w_{new}=\left[\frac{\partial^2 f}{\partial w^2}\right]^{1/2}\,w$.   Meanwhile, such a coordinate change does not change the successive $w_r$ computed by this idea algorithm because (1) it does not change the direction $d_r$ which depend only on the location of the minima $\hat{w}^*_p$, and (2) it does not change the line search termination conditions. Therefore, without changing the algorithm, we can, at each iteration, perform the analysis using the linear coordinate transform that yields the best contraction factor.  In other words, as it progresses towards the optimum, this \emph{ideal algorithm automatically adapts to the local curvature properties of the objective function.}

As already mentioned, it is not necessary for $w_p$ to be the minimizer of $\hat{f}_p$; we only need to find $w_p$ such that the direction $d_p = w_p-w^r$ satisfies (1).
The following result shows that if an optimizer with \emph{glrc} is used to minimize $\hat{f}_p$, then, only a constant number of iterations is needed to satisfy  the sufficient angle of descent condition.

Lemma 3

Theorem 4

Truncating the minimization of the local functions $\hat{f}_p$ accelerates the determination of the search directions $d^r$ but also compromises the algorithm invariance to linear coordinate transform, potentially losing the adaptive properties of the ideal algorithm.  In practice, experiments suggest that the benefit of truncation outweighs its posited drawbacks.
